# Supplementary material for: A Suite of Reduced-Order Models of a Single-Layer Lithium-ion Pouch Cell
Source: arXiv:2008.03691 source file (2020-08-09)
Supplement: Supplementary file 1 [file old_appendix.tex]

\begin{comment}

\section{Electrochemical Terms}\label{app:algebraic-expressions}

\subsection{Leading-order terms}
\begin{subequations}\label{eqn:leading-order-internals}
\begin{gather}
    N\ts{e,k}^0 = 0, \quad c\ts{e,k}^0 = 1, \quad \kin{n, s, p}, \\
    \phi\ts{s,n}^0 = \phi\ts{s,cn}, \quad \phi\ts{e,k}=\phi\ts{s,n}^0-\eta\ts{n}^0-U\ts{n}\left(c\ts{s,n}^0,T^0\right)\big|_{r\ts{n}=1}, \\
    \phi\ts{s,p}^0 = \phi\ts{s,n}^0 + U\ts{p}\left(c\ts{s,p}^0,T^0\right)\big|_{r\ts{p}=1} -U\ts{n}\left(c\ts{s,n}^0,T^0\right)\big|_{r\ts{n}=1}
    + \eta\ts{p}^0 - \eta\ts{n}^0, \\
    \eta\ts{n}^0 = 2(1 + \Theta T^0)\sinh^{-1}\left(\frac{\mathcal{I}^0}{j\ts{0,n}^0L\ts{n}} \right), \quad \eta\ts{p}^0 =-2 (1 + \Theta T^0)\sinh^{-1}\left(\frac{\mathcal{I}^0}{j\ts{0,p}^0L\ts{p}} \right).\\
    i\ts{e,n}^0 = x\frac{\mathcal{I}^0}{L\ts{n}}, \quad i\ts{e,s}^0=\mathcal{I}^0, \quad i\ts{e,p}^0 = (1-x)\frac{\mathcal{I}^0}{L\ts{p}}, \\
    \qquad j\ts{n}^0 = \frac{\mathcal{I}^0}{L\ts{n}}, \quad j\ts{p}^0 = -\frac{\mathcal{I}^0}{L\ts{p}}, \\
    j\ts{0,k}^0= \frac{\gamma\ts{k}}{\mathcal{C}\ts{r,k}} m\ts{k}(T^0) (c^0\ts{s,k})^{1/2} (1-c\ts{s,k}^0)^{1/2}.
\end{gather}
\end{subequations}

\subsection{First-order terms}

Electrolyte potentials:
\begin{subequations}
    \begin{align}
        &\phi\ts{e,n}^1 = \hat{\phi}\ts{e} + 2(1-t^+)(1 + \Theta T^0)c\ts{e,n}^1
        - \frac{\mathcal{I}^0}{\hat{\kappa}'\ts{e} \kappa\ts{e}(1, T^0)}\left(\frac{x^2-L\ts{n}^2}{2 \epsilon\ts{n}^{\text{b}} L\ts{n}} + \frac{L\ts{n}}{\epsilon\ts{s}^{\text{b}}} \right), \\
         &\phi\ts{e,s}^1 = \hat{\phi}\ts{e}  + 2(1-t^+) (1 + \Theta T^0)c\ts{e,s}^1
        - \frac{\mathcal{I}^0 x}{\hat{\kappa}'\ts{e} \kappa\ts{e}(1, T^0)\epsilon\ts{s}^{\text{b}}},\\
        &\phi\ts{e,n}^1 = \hat{\phi}\ts{e} + 2(1-t^+) (1 + \Theta T^0)c\ts{e,p}^1
        - \frac{\mathcal{I}^0}{\hat{\kappa}'\ts{e} \kappa\ts{e}(1, T^0)}\left(\frac{x(2-x)+L\ts{p}^2-1}{2\epsilon\ts{p}^{\text{b}} L\ts{p}} + \frac{1-L\ts{p}}{\epsilon\ts{s}^{\text{b}}} \right),\\
        & \hat{\phi}\ts{e} = - 2 (1+t^+) + \frac{\mathcal{I}^0}{\hat{\kappa}\ts{e}' \kappa\ts{e}(1, T^0)}\left(\frac{1}{3\epsilon\ts{n}^b} - \frac{1}{\epsilon\ts{s}^b} \right) + \Xav{\phi}\ts{s,n}^1 - \Xav{\eta}^1\ts{n} -\pdv{U\ts{n}}{c\ts{s,n}}(c\ts{s,n}^0, T^0)\Xav{c}\ts{s,n}^1 - \pdv{U\ts{n}}{T}(c\ts{s,n}^0, T^0)\Xav{T}^1,
    \end{align}
\end{subequations}
where the overbar represents $x$-electrode-averaged terms expressions for which are provided in Appendix \ref{app:electrode_averaged}.

Electrode solid-phase potentials:
\begin{subequations} \label{eqn:phisolid1}
\begin{align}
    &\phi\ts{s,n}^1 = \phi\ts{s,cn}^1 + \frac{\mathcal{I}^0x}{2\sigma\ts{n}' L\ts{n}}\left(2L\ts{n} - x\right), \\
    &\phi\ts{s,p}^1 = \phi\ts{s,cp}^1 +   \frac{\mathcal{I}^0 (x-1) (1-2L\ts{p}-x)}{2\sigma\ts{p}' L\ts{p}}.
\end{align}
\end{subequations}

Electrochemical reactions:
\begin{subequations}\label{eqn:od:all_BV}
    \begin{align} \label{eqn:od:BV}
        &j\ts{k}^1 = \frac{2 j\ts{k}^0 j\ts{0,k}^1}{j\ts{0,k}^0} + \frac{\eta\ts{k}^1\sqrt{(j\ts{0,k}^0)^2 + (j\ts{k}^0)^2}}{2(1+\Theta T^0)}
        - \frac{\Theta T^1 \sqrt{(j\ts{0,k}^0)^2 + (j\ts{k}^0)^2}\sinh^{-1}\left(\frac{j\ts{k}^0}{j\ts{0,k}^0}\right)}{1+\Theta T^0}, \\
    	\label{eqn:eta1}
    	&\eta\ts{k}^1 = \phi^1\ts{s,k} - \phi^1\ts{e,k} - \pdv{U\ts{k}}{c\ts{s,k}} (c\ts{s,k}^0,T^0) c\ts{s,k}^1\bigg|_{r\ts{k}=1} - \pdv{U\ts{k}}{T} (c\ts{s,k}^0,T^0)T^1\bigg|_{r\ts{k}=1},\\
        & j\ts{0,k}^1 = \frac{j\ts{0,k}^0}{2}\left(\frac{c\ts{s,k}^1}{c\ts{s,k}^0} - \frac{c\ts{s,k}^1}{1-c\ts{s,k}^0} + c\ts{e,k}^1 \right)\bigg|_{r\ts{k}=1} + \frac{j\ts{0,k}^0}{m\ts{k}(T^0)}m\ts{k}'(T^0)T^1\bigg|_{r\ts{k}=1}.
        \end{align}
\end{subequations}
% &j\ts{k}^1 = j\ts{0,k}^1 \sinh\left( \frac{\eta\ts{k}^0}{2(1 + \Theta T^0)}  \right) + \frac{j\ts{0,k}^0}{2}\left( \eta\ts{k}^1 - \frac{\Theta T^1}{(1 + \Theta T^0)}\right)\cosh(\frac{\eta\ts{k}^0}{2(1 + \Theta T^0)}), \\ % pretty sure this formula is wrong but leaving for reference

\clearpage

\section{X-Electrode-Averaged Quantities}\label{app:electrode_averaged}
\begin{align}
    % \label{eqn:av-c_neg}
	% &\bar{c}\ts{e,n}^1 = \frac{\mathcal{C}\ts{e}' (1-t^+) \mathcal{I}^0}{ 6\gamma\ts{e} D\ts{e}(1,T^0)}\left( 2\left(\frac{L\ts{p}^2}{\epsilon\ts{p}^{\text{b}}} - \frac{L\ts{n}^2}{\epsilon\ts{n}^{\text{b}}} \right) + \frac{2 L\ts{n}}{\epsilon\ts{n}^{\text{b}}} + \frac{3L_{s}}{\epsilon_{s}^{b}}(L\ts{p}-L\ts{n}+1)\right) \\
	% \label{eqn:av-c_pos}
    % &\bar{c}\ts{e,p}^1 = \frac{\mathcal{C}\ts{e}' (1-t^+) \mathcal{I}^0}{ 6\gamma\ts{e} D\ts{e}(1,T^0)}\left( 2\left(\frac{L\ts{p}^2}{\epsilon\ts{p}^{\text{b}}} - \frac{L\ts{n}^2}{\epsilon\ts{n}^{\text{b}}} \right) - \frac{2 L\ts{p}}{\epsilon\ts{p}^{\text{b}}} + \frac{3L_{s}}{\epsilon_{s}^{b}}(L\ts{p}-L\ts{n}-1)\right) \\
    &\Xav{\phi}\ts{e,n}^1 = \tilde{\phi}\ts{e} + 2(1-t^+)(1+\Theta T^0) \bar{c}\ts{e,n}^1 + \frac{\mathcal{I}^0L\ts{n}}{\hat{\kappa}\ts{e}' \kappa\ts{e}(1,T^0)}\left(\frac{1}{3 \epsilon\ts{n}^{\text{b}}} - \frac{1}{\epsilon_{s}^{\text{b}}}\right), \\
    &\bar{\phi}\ts{e,p}^1 = \tilde{\phi}\ts{e} + 2(1-t^+)(1+\Theta T^0) \bar{c}\ts{e,p}^1 + \frac{ \mathcal{I}^0L\ts{p}}{\hat{\kappa}\ts{e}' \kappa(1,T^0)}\left(\frac{1}{ \epsilon\ts{s}^{\text{b}}} - \frac{1}{3\epsilon\ts{p}^{\text{b}}}\right) - \frac{\mathcal{I}^0}{\hat{\kappa}\ts{e}' \kappa(1,T^0)\epsilon_{s}^{\text{b}}}, \\
    & \bar{\phi}\ts{s,n}^1 = \phi\ts{s,cn}^1 -\frac{\mathcal{I}^0L\ts{n}}{3 \sigma\ts{n}'}, \\
    &\bar{\phi}\ts{s,p}^1 =  \phi\ts{s,cp}^1  +\frac{\mathcal{I}^0L\ts{p}}{3 \sigma\ts{p}'}, \\
    &\bar{j}\ts{n}^1 = \frac{\mathcal{I}^1}{L\ts{n}}, \\
    &\bar{j}\ts{p}^1 = - \frac{\mathcal{I}^1}{L\ts{p}}, \\
    &\Xav{\eta}\ts{k}^1 = \frac{2(1+\Theta T^0)(j\ts{0,k}^0\Xav{j}\ts{k}^1 - j\ts{k}^0\Xav{j}\ts{0,k}^1)}{j\ts{0,k}^0\sqrt{(j\ts{0,k}^0)^2 + (j\ts{k}^0)^2}} + 2 \Theta \Xav{T}^1\sinh^{-1}\left(\frac{j\ts{k}^0}{j\ts{0,k}^0}\right)\quad\kin{n, p}.
    % &\Xav{\eta}\ts{k}^1 = \frac{2(1+\Theta T^0)(j\ts{k}^0\Xav{j}\ts{0,k}^1 + j\ts{0,k}^0\Xav{j}\ts{k}^1)}{j\ts{0,k}^0\sqrt{(j\ts{0,k}^0)^2 + (j\ts{k}^0)^2}} + 2 \Theta \Xav{T}^1\sinh^{-1}\left(\frac{j\ts{k}^0}{\frac{j\ts{0,k}^0}\right)
\end{align}

% pretty sure these are wrong but will leave them for reference
% &\Xav{\eta}\ts{k} = \frac{\Theta \Xav{T}^1}{(1+\Theta T^0)} + \frac{2 \left(\Xav{j}\ts{k}^1 - \Xav{j}\ts{0,k}^1\sinh\left( \frac{\eta\ts{k}^0}{2(1+\Theta T^0)}\right)\right)}{j\ts{0,k}\cosh\left(\frac{\eta\ts{k}^0}{2(1+\Theta T^0)}\right)}\\
% &\Xav{\eta}\ts{k} = \frac{\Theta \Xav{T}^1}{(1+\Theta T^0)} + \frac{2 \left(j\ts{0,k}^0\Xav{j}\ts{k}^1 - \Xav{j}\ts{0,k}^1j\ts{k}^0\right)}{j\ts{0,k}^0\sqrt{(j\ts{0,k}^0)^2 + (j\ts{k}^0)^2}}
\scott{We need to check the kappa prefactors. kappa tilde, kappa hat, kappa prime....}


\section{Heat generation terms}\label{app:heatgen}

\subsection{Definition}
\begin{subequations}\label{eqn:heat-gen-terms}
    \begin{align}
        Q\ts{k} &= Q\ts{Ohm,k} + Q\ts{rxn,k} + Q\ts{rev,k}  \quad && \kin{cn, n, s, p, cp},\\
    Q\ts{Ohm,k} &= - \left(\boldsymbol{i}\ts{s,k} \cdot\nabla\phi\ts{s,k} + \boldsymbol{i}\ts{e,k} \cdot\nabla \phi\ts{e,k}\right)&&\kin{n, p}, \\
            \label{eqn:thermal:ccs}
            Q\ts{Ohm,s} &= -\boldsymbol{i}\ts{e,s}\cdot\nabla\phi\ts{e,s}, \quad Q\ts{Ohm,k} = -\boldsymbol{i}\ts{s,k}\cdot\nabla\phi\ts{s,k} &&\kin{cn, cp},   \\
        \label{eqn:thermal:rxn}
        Q\ts{rxn,k} &=  j\ts{k} \eta\ts{k} &&\kin{n,p}, \\
        \label{eqn:thermal:rev}
        Q\ts{rev,k} &=  j\ts{k}(\Theta^{-1} + T\ts{k}) \pdv{U\ts{k}}{T\ts{k}}\bigg|_{T\ts{k}=0} &&\kin{n, p}.
    \end{align}
\end{subequations}

\subsection{Asymptotic expansions}
In each of the following limits, the combined leading- and first-order heat generation terms are given by
\begin{subequations}
    \begin{align}
        Q\ts{k}\co &= Q\ts{Ohm,k}\co + Q\ts{rxn,k}\co + Q\ts{rev,k}\co,\\
        Q\ts{Ohm,ck}\co &= Q\ts{Ohm,ck}^0 + \delta Q\ts{Ohm,ck}^1, \\
        Q\ts{Ohm,k}\co &= Q\ts{Ohm,k}^0 + \delta Q\ts{Ohm,k}^1, \\
        Q\ts{rxn,k}\co &= Q\ts{rxn,k}^0 + \delta Q\ts{rxn,k}^1, \\
        Q\ts{rev,k}\co &= Q\ts{rev,k}^0 + \delta Q\ts{rev,k}^1.
    \end{align}
\end{subequations}

\subsubsection{Limit of thin or low conducting current collectors and fast electrolyte diffusion}\label{app:low-conducting}
This limit is defined by the relations \eqref{eqn:thin-or-poorly-conducting-current-collectors}. In this limit the leading-order heat generation terms are
\begin{subequations}\label{eqn:thin-cc-leading-order-heating-terms}
    \begin{align}
        Q\ts{k}^0 &= Q\ts{Ohm,k}^0 + Q\ts{rxn,k}^0 + Q\ts{rev,k}^0,\\
        Q\ts{Ohm,ck}^0 &= \sigma\ts{ck}' \left\vert \nabla_\perp \phi\ts{s,ck}^0 \right\vert^2, \\
        Q\ts{Ohm,k}^0 &= 0, \\
        Q\ts{rxn,k}^0 &= j\ts{k}^0\eta\ts{k}^0, \\
        Q\ts{rev,k}^0 &= j\ts{k}^0(\Theta^{-1} + T^0)\Xi(c\ts{s,k}^0),
    \end{align}
\end{subequations}
and the first-order heat generation terms are
\begin{subequations}\label{eqn:thin-cc-first-order-heating-terms}
    \begin{align}
        Q\ts{k}^1 &= Q\ts{Ohm,k}^1 + Q\ts{rxn,k}^1 + Q\ts{rev,k}^1,\\
        Q\ts{Ohm,ck}^1 &= 2 \sigma\ts{ck}' \left\vert \nabla_\perp \phi\ts{s,ck}^0 \right\vert \left\vert \nabla_\perp \phi\ts{s,ck}^1 \right\vert , \\
        Q\ts{Ohm,k}^1 &= -i\ts{s,k}^0\pdv{\phi\ts{s,k}^1}{x} - i\ts{e,k}^0\pdv{\phi\ts{e,k}^1}{x}, \\
        Q\ts{rxn,k}^1 &= j\ts{k}^0\eta\ts{k}^1 + j\ts{k}^1\eta\ts{k}^0,\\
        Q\ts{rev,k}^1 &= (\Theta^{-1} + T^0)\Xi\ts{k}(c\ts{s,k}^0)j\ts{k}^1 + j\ts{k}^0\Xi\ts{k}(c\ts{s,k}^0)T^1 + j\ts{k}^0(\Theta^{-1} + T^0)\Xi\ts{k}'(c\ts{s,k}^0)c\ts{s,k}^1.
    \end{align}
\end{subequations}
where
 \begin{equation}
    \Xi\ts{k}(c\ts{s,k}) = \pdv{U\ts{k}}{T}\bigg\vert_{T=0} (c\ts{s,k}).
\end{equation}
\end{comment}


\begin{comment}
\begin{subequations}\label{eqn:thin-cc-heating-terms}
\begin{align}
    Q\ts{Ohm,ck} &=  \sigma\ts{ck}' \left\vert \nabla_\perp \phi\ts{s,ck}^0 \right\vert^2 + 2 \delta\sigma\ts{ck}' \left\vert \nabla_\perp \phi\ts{s,ck}^0 \right\vert \left\vert \nabla_\perp \phi\ts{s,ck}^1 \right\vert + \cdots, \\
    \nonumber
    Q\ts{Ohm,k} &= -\left( \left( i\ts{s,k}^0 + \delta i\ts{s,k}^1 + \cdots \right) \left( \pdv{\phi\ts{s,k}^0}{x} + \delta \pdv{\phi\ts{s,k}^1}{x} + \cdots \right) + \left( i\ts{e,k}^0 + \delta i\ts{e,k}^1 + \cdots \right) \left( \pdv{\phi\ts{e,k}^0}{x} + \delta \pdv{\phi\ts{e,k}^1}{x} + \cdots \right)   \right) \\
    &= -\delta\left( i\ts{s,k}^0\pdv{\phi\ts{s,k}^1}{x} + i\ts{e,k}^0\pdv{\phi\ts{e,k}^1}{x}\right) + \cdots, \qquad \qq{since}  \pdv{\phi\ts{s,k}^0}{x} =  \pdv{\phi\ts{e,k}^0}{x} = 0, \\
    Q\ts{rxn,k} &= j\ts{k}^0\eta\ts{k}^0 + \delta(j\ts{k}^0\eta\ts{k}^1 + j\ts{k}^1\eta\ts{k}^0) + \cdots, \\
    \nonumber
    Q\ts{rev,k} &= j\ts{k}^0(\Theta^{-1} + T^0)\Xi\ts{k}(c\ts{s,k}^0) \\
    & \qquad + \delta \left[ (\Theta^{-1} + T^0)\Xi\ts{k}(c\ts{s,k}^0)j\ts{k}^1 + j\ts{k}^0\Xi\ts{k}(c\ts{s,k}^0)T^1 + j\ts{k}^0(\Theta^{-1} + T^0)\Xi\ts{k}'(c\ts{s,k}^0)c\ts{s,k}^1 \right],
\end{align}
\end{subequations}
is the entropic heat coefficient, which is a function of concentration $c\ts{s,k}$.
\end{comment}

\begin{comment}
\subsubsection{The limit of high current collector conductance}\label{app:high-no-diff}
This limit is defined by the relations \eqref{eqn:highly-conducting-current-collectors}. In this limit, the leading-order heating terms are the same as those in \eqref{eqn:thin-cc-leading-order-heating-terms} but with the Ohmic heating in the current collectors, electrodes, and electrolyte, replaced by
\begin{subequations}
    \begin{align}
        Q\ts{Ohm,ck}^0 &= 0, \\
        Q\ts{Ohm,k}^0 &= \sigma\ts{k} \left\vert \nabla_\perp \phi\ts{s,k}^0 \right\vert^2.
    \end{align}
\end{subequations}
The first-order heating terms are also the same as those in \eqref{eqn:thin-cc-first-order-heating-terms} but with the Ohmic heating in the current collectors, electrodes, and electrolyte replaced by
\begin{subequations}
    \begin{align}
        Q\ts{Ohm,ck}^1 &= \sigma\ts{ck}'' \left\vert \nabla_\perp \phi\ts{s,ck}^1 \right\vert^2, \\
        Q\ts{Ohm,k}^1 &= -i\ts{s,k}^0\pdv{\phi\ts{s,k}^1}{x} -i\ts{e,k}^0\pdv{\phi\ts{e,k}^1}{x}
                         -i\ts{s,k}^1\pdv{\phi\ts{s,k}^0}{x} -i\ts{e,k}^1\pdv{\phi\ts{e,k}^0}{x}
    \end{align}
\end{subequations}
\end{comment}

%\subsection{Limit of high current collector conductance}\label{app:high-with-diff}
%This limit is defined by the relations in \eqref{eqn:highly-conducting-with-fast-diffusion}. In this limit, the leading-order heating terms are the same as those in \eqref{eqn:thin-cc-leading-order-heating-terms} but with the Ohmic heating in the current collectors replaced by
%\begin{equation}
    %Q\ts{Ohm,ck}^0 = 0.
%\end{equation}
%The first-order heating terms are also the same as those in \eqref{eqn:thin-cc-first-order-heating-terms} but with the Ohmic heating in the current collectors replaced by
%\begin{equation}
    %Q\ts{Ohm,ck}^1 = \sigma\ts{ck}'' \left\vert \nabla_\perp \phi\ts{s,ck}^1 \right\vert^2.
%\end{equation}

\begin{comment}

\subsection{Calculation of averaged heat generation terms required for the SPMeCC}
For the SPMeCC we require the $x$-avergaed leading-order heat source term and volume-averaged first order correction. These are calculated to be
\begin{align}
\nonumber
    L\bar{Q}_0 &= \frac{I\ts{app}}{L_y}\left[ 2(1+\Theta T^0) \sinh^{-1}\left(\frac{I_{\text{app}}}{\bar{j}\ts{0,n}^0 L\ts{n} L_y}\right) + (\Theta^{-1} + T^0)\left.\pdv{U\ts{n}}{T}\right|_{T=0} \right] \\
    &\quad +  \frac{I\ts{app}}{L_y}\left[2 (1+\Theta T^0) \sinh^{-1}\left(\frac{I_{\text{app}}}{\bar{j}\ts{0,p}^0 L\ts{p} L_y}\right) - (\Theta^{-1} + T^0)\left.\pdv{U\ts{p}}{T}\right|_{T=0} \right] \\
    \nonumber
    L\tilde{\bar{Q}}^1 &= I\ts{app}^2\frac{\sigma\ts{cn}''L\ts{cn}}{L_y} \int_0^1 \int_0^{L_y} \left| \frac{\nabla_\perp\psi + (\alpha'/L_y)\sigma\ts{cp}''L\ts{cp}\nabla_\perp \mathcal{W}^1}{\sigma\ts{cn}''L\ts{cn} + \sigma\ts{cp}''L\ts{cp}} \right|^2 \dd{y} \dd{z} \\
    \nonumber
    &\quad + I\ts{app}^2\frac{\sigma_{cp}''L\ts{cp}}{L_y} \int_0^1 \int_0^{L_y}  \left| \frac{\nabla_\perp\psi - (\alpha'/L_y)\sigma_{cn}''L\ts{cn}\nabla_\perp \mathcal{W}^1}{\sigma_{cn}''L\ts{cn} + \sigma_{cp}''L\ts{cp}} \right|^2 \dd{y} \dd{z} \\
    \nonumber
    &\quad + \left(\frac{I\ts{app}}{L_y}\right)^2 \frac{L\ts{n}}{3\sigma\ts{n}'} -  \left(\frac{I\ts{app}}{L_y}\right)\int_0^{L\ts{n}} \frac{x}{L\ts{n}}\pdv{\phi\ts{e,n}^1}{x} \dd{x} + \mathcal{I}^0\tilde{\bar{\eta}}\ts{n}^1 + \mathcal{I}^0 \tilde{T}^1 \left.\pdv{U\ts{n}}{T}\right|_{T=0} \\
    \nonumber
    &\quad - \frac{I\ts{app}}{L_y}\int_{L\ts{n}}^{1-L\ts{p}} \pdv{\phi\ts{e,p}^1}{x} \dd{x}\\
    \label{eqn:volumeav:Q1}
    &\quad + \left(\frac{I\ts{app}}{L_y}\right)^2 \frac{L\ts{p}}{3\sigma\ts{p}'} -  \left(\frac{I\ts{app}}{L_y}\right)\int_{1 - L\ts{p}}^1\frac{1-x}{L\ts{p}}\pdv{\phi\ts{e,p}^1}{x} \dd{x} - \mathcal{I}^0\tilde{\bar{\eta}}\ts{p}^1 - \mathcal{I}^0 \tilde{T}^1 \left.\pdv{U\ts{p}}{T}\right|_{T=0},
\end{align}
where the terms \eqref{eqn:volumeav:Q1} in correspond to Ohmic heating in the negative current collector, Ohmic heating in the positive current collector, Ohmic heating in the negative electrode, reaction heating in the negative electrode, reversible heating in the negative electrode, Ohmic heating in the separator, Ohmic heating in the positive electrode, reaction heating in the positive electrode, and reversible heating in the positive electrode.  The integrals in the electrolyte Ohmic heating above may be computed explicitly, but are left in the integral form above for compactness. In the above, the volume-averaged overpotentials are
\begin{equation}
    \tilde{\bar{\eta}}\ts{k}^1 = - \frac{2\tilde{\bar{j}}\ts{0k}^1}{j\ts{0,k}^0  L\ts{k}}\tanh{\left(\frac{\Lambda\eta\ts{k}^0}{2(1 + \Theta T^0)}\right)} + \frac{\Theta\tilde{T}^1}{1 + \Theta T^0}.
\end{equation}
\end{comment}
